# Supplementary material for: Electronic excitation spectra of molecular hydrogen in Phase I from Quantum Monte Carlo and Many-Body perturbation methods
Source: arXiv:2311.08506 source file (2024-05-20)
Supplement: Supplementary file 1 [file Supplementary_Material__Electronic_excitation_spectra_of_molecular_hydrogen_in_Phase_I_from_Quantum_Monte_Carlo_and_Many_Body_perturbation_methods_.pdf]

# Supplementary Material: Electronic excitation spectra of molecular hydrogen in Phase I from Quantum Monte Carlo and Many-Body perturbation methods.

Vitaly Gorelov
*Laboratoire des Solides Irradiés, École Polytechnique, CNRS, CEA/DRF/IRAMIS, Institut Polytechnique de Paris, F-91128 Palaiseau, France. and European Theoretical Spectroscopy Facility (ETSF)*

Markus Holzmann
*Univ. Grenoble Alpes, CNRS, LPMMC, 38000 Grenoble, France*

David M. Ceperley
*Department of Physics, University of Illinois Urbana-Champaign, Urbana, Illinois 61801, USA*

Carlo Pierleoni
*Department of Physical and Chemical Sciences, University of L'Aquila, Via Vetoio 10, I-67010 L'Aquila, Italy*
(Dated: May 20, 2024)

## SUPPLEMENTARY MATERIAL

### Equation of state and generation of nuclear configurations

In this section we report our results for the equilibrium sampling of the system. As stated in the main text, we prepare the supercell of 48 molecules with the molecular centers on an hcp structure with a $c/a$ ratio using the experimental measurements [1]. The molecular bond lengths were set to be $1.4\mathring{A}$ with bond directions randomly oriented over the sphere. The configurations were relaxed at constant pressure using Quantum Espresso with the vdW-DF1 functional. The procedure was repeated for four different pressure values at zero temperature: $P_{vdW-DF1}(T=0) = 5,\ 10,\ 50,\ 90$ GPa. After geometry optimization we performed NVT-Smart Monte Carlo simulation at T=300K employing energies and forces using the vdW-DF1 functional to sample the equilibrium distribution of the system and generate a set of statistically uncorrelated configurations for the energy gap calculation. For each system, trajectories of at least 20000 global MC steps after equilibration have been generated. This procedure was repeated at four different densities corresponding to $r_s = 2.211, 1.968, 1.706, 1.589$ to investigate the pressure range between 5GPa and 90GPa. Nuclear quantum effects, important in high pressure hydrogen, are considered by representing protons as Path Integrals. In this case convergence in imaginary time for room temperature protons was achieved with 16 time slices. The pressures were obtained by averaging over configurations. Comparison of the computed pressure values with the experimental Equation of State (EOS) is reported in figures 1 and 2. To determine a reference EOS we use a Vinet fit to the experimental data up to 120GPa [1]

$$P_{exp} = 3\,K_0 x^{2/3}\left[1-\frac{1}{x^{1/3}}\right]\exp\left\{\frac{3}{2}(K_0'-1)\left[1-\frac{1}{x^{1/3}}\right]\right\} \quad (1)$$

where $x = V_0/V = (r_{s_0}/r_s)^3 = \rho/\rho_0$ with $V_0 = 25.433cm^3/mol = 285.29a_0^3$ corresponding to $r_{s_0} = 3.2413$, $K_0 = 0.162GPa$ and $K_0' = 6.813$. The values of $P_{exp}$ for the four different compressions considered here are given in table I. All pressure values, $P$, quoted in the following, as well as in the main text, refer to the reference EOS, $P_{exp}$, if not explicitly stated otherwise.

In figures 1 and 2 we plot the deviation of the computed EOS from experiments for vdW-DF1, PBE and RQMC electronic structure methods using both classical and quantum protons. For classical protons vdW-DF1 EOS is systematically above the reference, while PBE and RQMC are systematically below the reference, PBE being slightly closer to the reference. The same picture is observed for quantum protons but now the PBE and RQMC are much closer to the reference pressures with a maximum deviation of about 2.5GPa in the intermediate pressure range. Relative deviations of RQMC pressures from the reference range from about 20% at low compression to below 1% at nine-fold compression when quantum nuclear effects are included.

X-ray diffraction experiments provide the $c/a$ ratio of the m-HCP structure [1]. In figure 3 we compare our relaxed cell geometry with the experimental data. We plot $c/a$ versus pressure for quantum protons in order to show the sensitivity of these data to the various electronic structure methods. We observe agreement of our data within the experimental error bars except at the second pressure where the deviation is about two standard deviations. The theoretical slope is smaller than the experimental one and this difference is due to the inaccuracy of the vdW-DF1 force field and of the adopted procedure of performing geometry optimization in ab-

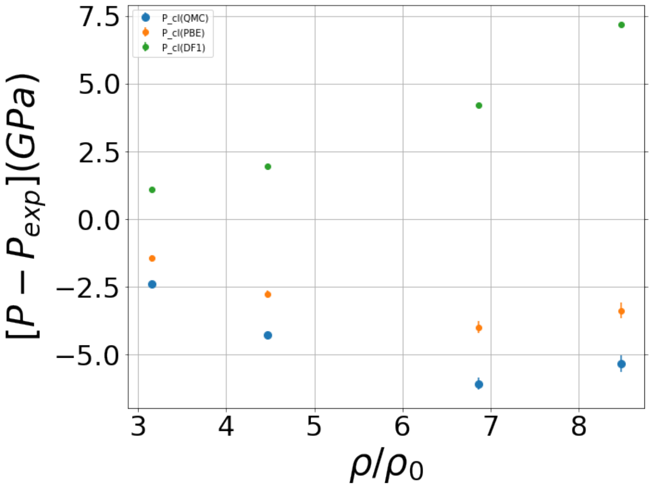


FIG. 1. Deviation of the calculated pressure from the experimental pressure as a function of compression computed using vdW-DF1 (green circles), PBE (orange circles) and RQMC (blue circles). All computed with classical protons.

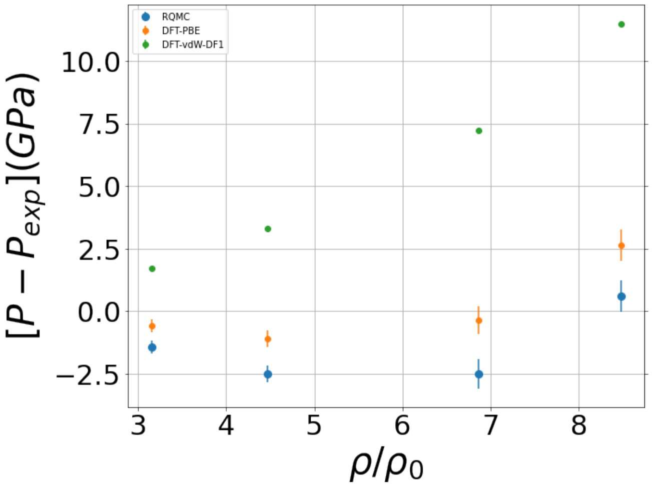


FIG. 2. Quantum proton systems. Deviation of the calculated pressure from the experimental pressure as a function of compression computed using vdW-DF1 (green circles), PBE (orange circles) and RQMC (blue circles). All computed with quantum protons.

sence of nuclear thermal and quantum effects. An optimal procedure would be to perform a constant pressure calculation with the QMC electronic energies and forces in presence of quantum protons within the path integral representation, a procedure doable but not yet available. Nonetheless, we believe that the observed inaccuracy in pressure and $c/a$ ratio only introduces a small bias in our study.

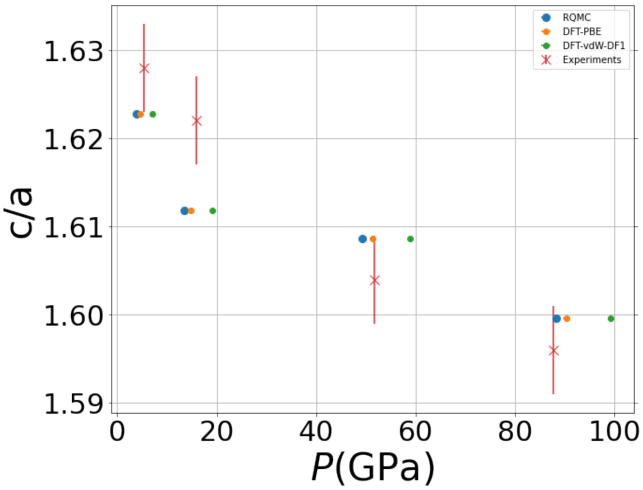


FIG. 3. The $c/a$ ratio computed with RQMC, vdW-DF1 and PBE compared with experimental measurements versus pressure. Since calculations are performed in a fixed supercell, the difference between the various calculations are with respect to computed pressures. Calculations assumed quantum protons.

## Quantum Monte Carlo calculations (QMC)

### *Electronic energies*

All electronic QMC calculations in this work used a Slater-Jastrow trial wave function including backflow (BF) [2, 3]. The Jastrow and BF functions were fully optimized within variational Monte Carlo, including the long-range (reciprocal lattice) contributions. The orbitals in the Slater determinant were from DFT-PBE calculations using Quantum Espresso [4, 5], which has been shown to provide a good trial QMC wave function [6, 7]. Since we are interested in the spin-neutral charge gap, we used an equal number of spin-up and spin-down electrons. We used a $6\times6\times6$ twist grid. Electronic energies were obtained with Reptation QMC (RQMC) using an imaginary time step of 0.01 $H^{-1}$ and a projection time of 2 $H^{-1}$.

The fundamental gap was obtained by grand-canonical twist averaged RQMC as described in [8]. The trace over nuclear configuration was performed by the quantum averaging procedure described in [9, 10]. The electronic energy levels are first averaged over nuclear degrees of freedom. The electronic gap is then determined by the minimum between nuclear averaged excitation energies. This is in contrast to the semiclassical approximation where the gap is attributed to a single nuclear configuration with the minimum electronic excitation[11, 12]. For more details see the SM of ref. [9] and ref. [10].

Quantum averaging over nuclear configurations was also employed for determining the neutral gap. In practice, for a fixed twist and nuclear configuration excited

states were obtained by promoting a single electron from the lowest energy state to the next level, according to the DFT eigenvalues. Neutral excitation energies were then obtained from RQMC calculation an then averaged over nuclear configurations. The neutral gap corresponds to the twist with the minimum excitation energy. This procedure extends the neutral gap calculation for ideal crystal structures [13] to quantum thermal crystals. Note that with the assumption of DFT orbitals in the trial function, a possible particle-hole interaction is not taken into account.

*Size effects*

Corrections of quasiparticle and neutral gaps due to the finite size of our simulation cell are based on the procedure discussed in Ref. [8] and [13], analysing the behavior of the static structure factors, $S_{N_e}(k)$, at fixed simulation cells, in the limit of $k \to 0$ thus avoiding extrapolation using different supercells. In the following, we discuss in more detail the size corrections.

The middle columns of figure 4 show the change in the static structure factor as two electrons (upper curves) or holes (lower curves) are added to the insulating system with $N$ atoms

$$S_k^{\pm} \equiv \frac{1}{2}(N_e \pm 2) S_{N_e \pm 2}(k) - \frac{1}{2} N_e S_{N_e}(k). \quad (2)$$

As discussed in [8] the inverse dielectric constant (shown as black horizontal line) can be extracted as:

$$\frac{1}{\epsilon} \approx \lim_{k \to 0} (S_k^+ + S_k^-). \quad (3)$$

Size effects on the quasi-particle gaps are then obtained by $|v_M(L)|/\epsilon$, e.g. Eq. 3 of the main text in the limit of $l_X \to \infty$ where localization effects vanish (see for instance refs [13, 15, 16]).

Size effects increase the quasi-particle gap compared to the bare results from the supercell calculations. However, the precise value of $1/\epsilon$ depends on the parameters and ranges used in the fitting procedure. An independent bound of the dielectric constant can be obtained from the structure factor of the insulating system in its electronic ground state [17, 18]

$$S_{N_e}(k) \leq \frac{\hbar k^2}{2m\omega_p} \left(1 - \frac{1}{\epsilon_k}\right)^{1/2}. \quad (4)$$

By inverting this equation for $1/\epsilon_k$ we extrapolate $1 - \Gamma_k^2$ (with $\Gamma_k \equiv 2m\omega_p S_{N_e}(k)/\hbar k^2$) to $k = 0$ and obtain an upper bound to the inverse dielectric constant. On the left column of Fig. 4 we show how this inequality holds for the dielectric constant extracted from Eq. 3. Benchmark calculations on Si and diamond C [8] have found a remarkable agreement of the value of the bound compared to experiment, which would indicate that our size effects for the quasi-particle gap based on extrapolating Eq. (3) might underestimate the true ones.

Concerning size effects of the neutral gap (Eq. 3 of the main text) we also have to estimate the length scale, $l_x = \epsilon/\mu$, where electron-hole attraction sets in [13]. Therefore, we need an estimate of the effective electron-hole mass, $\mu$, of neutral particle-hole excitations. This can be obtained from the dependence of the electron-hole excitation energy on the twist angle of the boundary conditions. On the right column of figure 4 the values of $\Delta_n(\mathbf{k}) = E_1(N_e, \mathbf{k}) - E_0(N_e, \mathbf{k})$ are resolved along $y$ and $z$ directions around $k = 0$. Despite large statistical uncertainties, it is possible to fit a parabola around a minimum at $\mathbf{k} = 0$ from which the values of $1/2\mu$ are extracted as prefactors and reported in table I. Due to the layered structure, excitations are primarily in the x-y plane, and since in $x$ direction only positive directions are available, we use $y$ direction to extract the electron-hole effective mass.

Because we just need those numbers for an order of magnitude estimate, we did not attempt to estimate the residual finite size bias of the effective electron-hole mass.

Table I summarises all quantities extracted from figure 4 (effective band mass, dielectric constant, excitation length) for the four compressions. We also provide the dielectric constant extracted from BSE (see below) averaged over independent configurations. In MBPT exciton binding energies correspond to the difference between BSE and GW gap while in QMC to the difference between quasiparticle and neutral gaps. Table II provides the QMC quasiparticle and neutral gaps obtained in the simulation cell with 96 electrons and the gaps extrapolated to the infinite cell size limit using the schemes described here and in Eq. (3) of main text.

When $2\ell_X$ is comparable or smaller than the simulation cell, particles and holes can form localized states (excitons). However, the use of extended orbitals from a plane wave basis in single determinant-QMC calculations prevents a direct observation of excitons even at the lowest compression. In order to have an exciton, we performed QMC calculations using Gaussian orbitals in the Slater determinant. For each molecule, we built molecular orbitals from a linear combination of two Gaussians, each centered at the atomic positions in a molecule. The ground state is built with the symmetric state (bonding) while in the excited state, one electron of the molecule with the longest bond is promoted into an antibonding state. The calculated optical gap at lowest compression is in quantitative agreement with the corresponding value from the extended DFT orbitals. The energies of the ground and the excited states are above the corresponding energies obtained with extended DFT orbitals by about 1 mHa per electron. Even though the wave function based on DFT orbitals gives lower energies, we

TABLE I. Compression $\rho/\rho_0$, pressure, electron-hole mass $\mu^{QMC}$, Madelung constant $v_M$, excitation length $l_X = \epsilon/\mu$ and the shortest of the three supercell dimensions $L = \min\{L_x, L_y, L_z\}$. $\epsilon^{S_k}$ and $\epsilon^{bound}$ are the dielectric constants extracted from the fits to QMC data shown on the middle and left columns of Fig. 4, based on Eqs. (3),(4) respectively, $\epsilon^{BSE}$ refers to the value obtained within BSE, the experimental dielectric constant at zero pressure is 1.28 [14]. $E_b^{QMC}$ and $E_b^{BSE}$ are the binding energies calculated in QMC and BSE respectively. Estimates of the uncertainty are provided in brackets (...). QMC values are given for cells with 96 electrons.

| $\rho/\rho_0$ | P (GPa) | $\mu^{QMC}$ | $l_X^{QMC}$ (Bohr) | $L$ (Bohr) | $v_M$ (Hartree) | $\epsilon^{S_k}$ | $\epsilon^{bound}$ | $\epsilon^{BSE}$ | $E_b^{BSE}$ (eV) | $E_b^{QMC}$ (eV) |
|---|---|---|---|---|---|---|---|---|---|---|
| 8.48 | 87 | 0.4(1) | 20(6) | 10.94 | 0.24 | 8.0(6) | 4.4(1) | 4.7(1) | 0.53(6) | 0.4(3) |
| 6.86 | 51 | 0.4(2) | 13(4) | 11.73 | 0.22 | 5.7(4) | 3.48(5) | | | 0.6(3) |
| 4.47 | 16 | 0.5(2) | 7(2) | 13.52 | 0.19 | 3.5(1) | 2.39(2) | 2.49(2) | 1.41(4) | 1.8(3) |
| 3.15 | 5 | 0.6(4) | 4(3) | 15.16 | 0.17 | 2.5(1) | 1.90(1) | 1.56(1) | 2.11(5) | 2.4(3) |

TABLE II. Quasiparticle $\Delta_{qp}^L$ and neutral $\Delta_n^L$ QMC gaps as obtained for the finite size cell with 96 electrons and their values $\Delta_{qp}^\infty$ and $\Delta_n^\infty$ extrapolated to the infinite simulation cell extrapolation limit. Brackets (...) indicate estimates of the uncertainty in the last digit dominated by the statistical average over configurations.The uncertainties arising from variations in dielectric constant and exciton extension length are statistically insignificant compared to the gaps' uncertainties for each pressure, except at the second compression level of $\rho/\rho_0 = 6.86$. There, we denote the systematic shift due to size effect errors using superscripts and subscripts.

| $\rho/\rho_0$ | $\Delta_{qp}^L$ (eV) | $\Delta_{qp}^\infty$ (eV) | $\Delta_n^L$ (eV) | $\Delta_n^\infty$ (eV) |
|---|---|---|---|---|
| 8.48 | 5.5(3) | 6.3(3) | 5.4(1) | 6.0(1) |
| 6.86 | 6.7(3) | 7.6(3) | 6.6(1) | $7.2^{7.3}_{7.0}(1)$ |
| 4.47 | 8.9(3) | 10.5(3) | 8.6(1) | 8.6(1) |
| 3.15 | 10.5(3) | 12.2(3) | 9.7(1) | 9.7(1) |

can use the results of the Gaussian orbitals to model the effects of localization, in particular on the structure factors used to estimate finite size effects.

For comparison, Figure 5 shows the difference $\Delta S(k) \equiv S_1(k) - S_0(k)$ between excited and ground state structure factors for the neutral gap calculation at $\rho/\rho_0 = 3.15$ using (extended) Bloch orbitals (left panel) and (localized) Gaussian orbitals (right panel). In the case of Gaussian orbitals the difference extrapolates to zero at vanishing momentum $k$, indicating no size effects, as one expects due to the localized character of the orbitals. In the case of extended Bloch orbitals $\Delta S(k)$ extrapolates to a slightly lower value than the one observed for quasi-particle excitations at the corresponding compression, which is due to electron-hole correlations (see Fig. 4).

## Many-Body Perturbation Theory (MBPT)

### *Optical spectra calculations*

Electronic excitations spectra [19] of $H_2$ crystals have been calculated using the Bethe-Salpeter equation [20] (BSE) in the framework of many-body perturbation theory [17] (MBPT).

In reciprocal space, the longitudinal inverse microscopic dielectric function $\epsilon^{-1}_{\mathbf{G},\mathbf{G}'}(\mathbf{q},\omega)$ is a matrix in the reciprocal lattice vectors $\mathbf{G}$ and $\mathbf{G}'$, and function of the frequency $\omega$ and the first-Brillouin-zone wavevector $\mathbf{q}$. The macroscopic dielectric function is obtained by averaging over the volume. This is equivalent to taking the $\mathbf{G} = 0$ limit [21, 22]:

$$\epsilon_M(\mathbf{q},\omega) \equiv \epsilon_1(\mathbf{q},\omega) + i\epsilon_2(\mathbf{q},\omega) = \frac{1}{\epsilon^{-1}_{\mathbf{G}=\mathbf{G}'=0}(\mathbf{q},\omega)}. \quad (5)$$

The optical absorption spectrum is given by the long-wavelength limit: $\epsilon_2(\omega) = \lim_{\mathbf{q}\to 0} \epsilon_2(\mathbf{q},\omega)$, whereas the loss function, measured by inelastic x-ray scattering (IXS) technique or electron energy loss spectroscopy (EELS), as a function of the momentum transfer $\mathbf{q}$ is given by $-\mathrm{Im}\,\epsilon_M^{-1}(\mathbf{q},\omega)$. By expressing the loss function in terms of the real and imaginary parts of the dielectric function one has:

$$-\mathrm{Im}\,\epsilon_M^{-1}(\mathbf{q},\omega) = \frac{\epsilon_2(\mathbf{q},\omega)}{[\epsilon_1(\mathbf{q},\omega)]^2 + [\epsilon_2(\mathbf{q},\omega)]^2}. \quad (6)$$

The loss function at vanishing momentum is a tensor that depends on the direction of $\mathbf{q}$. To account for the random orientation of hydrogen crystals in the experiment we plot the average over the three directions:

$$-\frac{1}{3}\mathrm{Im}\Big( \lim_{\substack{q_x\to 0\\ q_y=0\\ q_z=0}} \epsilon_M^{-1}(\mathbf{q},\omega) + \lim_{\substack{q_x=0\\ q_y\to 0\\ q_z=0}} \epsilon_M^{-1}(\mathbf{q},\omega) + \lim_{\substack{q_x=0\\ q_y=0\\ q_z\to 0}} \epsilon_M^{-1}(\mathbf{q},\omega)\Big) \quad (7)$$

Within MBPT, the quasiparticle (QP) addition and removal energies that form the band structures of materials can be obtained from the poles of the one-particle Green's function $G(\mathbf{r},\mathbf{r}',\omega)$. The effects of the electron-electron interaction beyond the electrostatic Hartree potential are encoded in the self-energy $\Sigma_{\mathrm{xc}}(\mathbf{r},\mathbf{r}',\omega)$. In

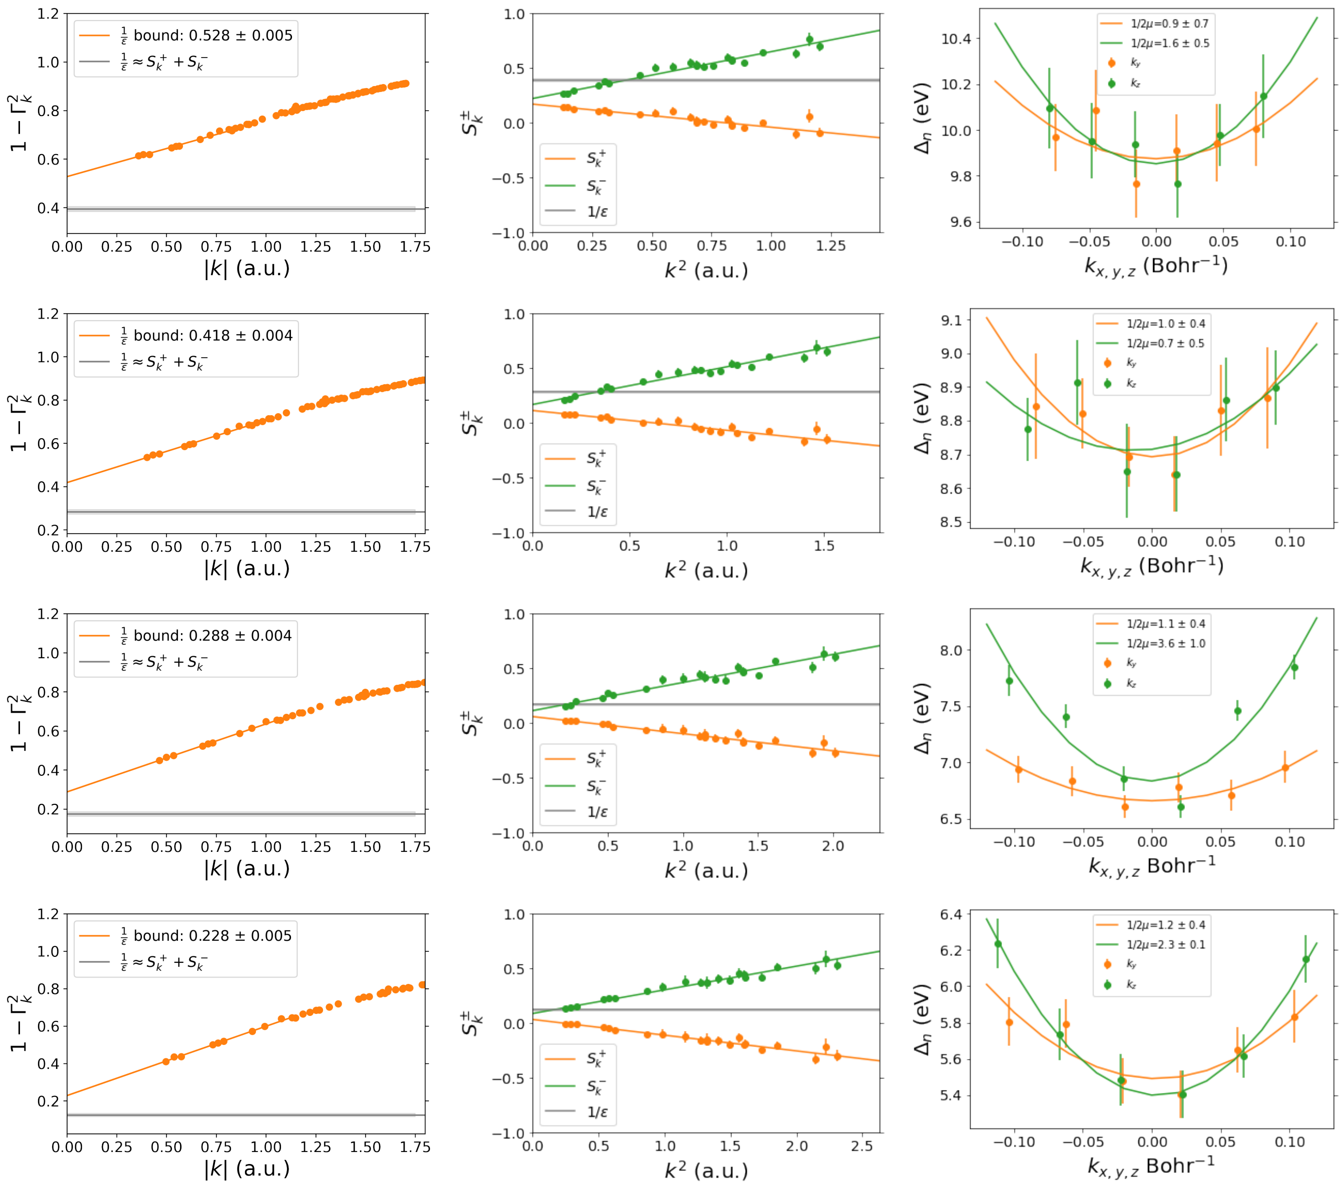

FIG. 4. Left: Upper bounds to the inverse dielectric constant Eq. (4), where $\Gamma_k \equiv 2m\omega_p S_{N_e}(k)/\hbar k^2$ (we include 10 first points in the linear extrapolation fit). Middle: Electron removal ($S_k^-$) and addition ($S_k^+$) structure factors which for $k \to 0$ tend to the inverse dielectric constant shown as the black horizontal line (extracted from the linear fit, all the points shown are included in the fit). Right: The dispersion of the quasiparticle gap around its minimum in two directions: $k_y$ ( orange) and $k_z$ (green). From top to bottom: $\rho/\rho_0 = 3.15, 4.47, 6.86, 8.48$ respectively.

the GW approximation [23] (GWA), $\Sigma_{\rm xc}(\omega)$ is given by the convolution between $G(\omega)$ and the screened Coulomb interaction $W(\omega) = \epsilon^{-1}(\omega)v_c$ evaluated in the RPA. In the $G_0W_0$ scheme [24, 25], the Kohn - Sham (KS) Green's function is used to build the RPA $W_0$ and the self-energy.

Approximations for solving the BSE in materials are available that yield exciton properties of materials accurately [26–29]. In particular, in the GWA with a statically screened Coulomb interaction $W$, the BSE can be reformulated as an electron-hole (excitonic) Hamiltonian problem: $H_{\rm exc}A_\lambda = E_\lambda A_\lambda$. In the basis $|v c\mathbf{k}\rangle$ of resonant transitions between occupied $v\mathbf{k}$ and unoccupied states $c\mathbf{k}$, and neglecting the coupling with antiresonant transitions (the Tamm-Dancoff approximation), the excitonic Hamiltonian reads:

$$\langle vc\mathbf{k}|H_{\rm exc}|v'c'\mathbf{k}'\rangle = E_{vc\mathbf{k}}\delta_{vv'}\delta_{cc'}\delta_{\mathbf{k}\mathbf{k}'} + \langle vc\mathbf{k}|\bar{v}_c - W|v'c'\mathbf{k}'\rangle. \quad (8)$$

Here $E_{vc\mathbf{k}} = E_{c\mathbf{k}} - E_{v\mathbf{k}}$ are the GWA transition energies between occupied and empty states, while the electron-hole interaction matrix elements are the sum of the attractive direct electron-hole interaction $-W$ and the re-

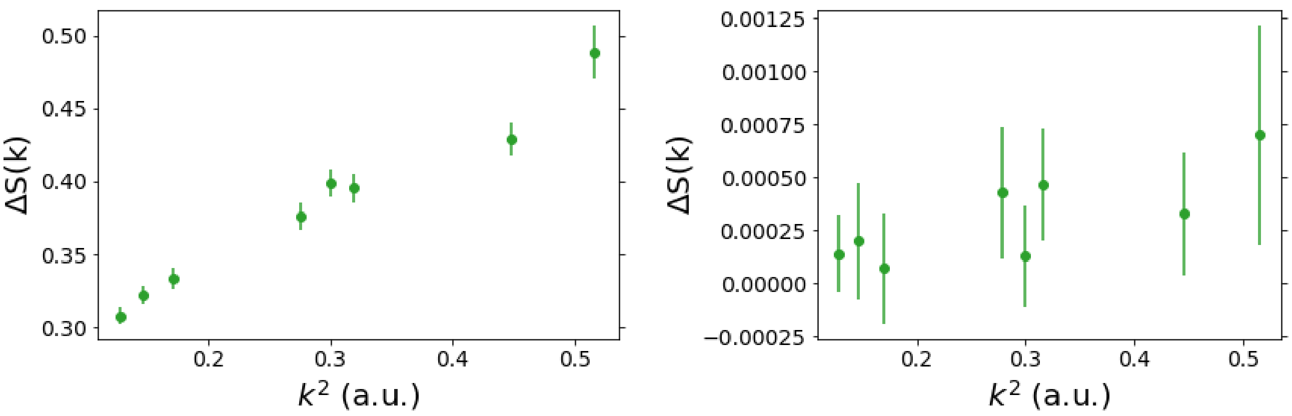


FIG. 5. $\Delta S(k) = S_1(k) - S_0(k)$ for a neutral excitation at $\rho/\rho_0 = 3.15$. Left: with Bloch orbitals. Right: with Gaussian orbitals.

pulsive electron-hole exchange interaction $\bar{v}_c$ given by the microscopic components (i.e., $\mathbf{G} \neq 0$) of the bare Coulomb interaction. In the Tamm-Dancoff approximation, which is usually a good approximation for semiconductors and insulators [19], the macroscopic dielectric function is obtained from the eigenvectors $A_\lambda^{vc\mathbf{k}}$ and eigenvalues $E_\lambda$ of the excitonic hamiltonian as:

$$\epsilon_M(\mathbf{q},\omega) = 1 - \lim_{\mathbf{q}\to 0} \frac{8\pi}{\Omega q^2} \sum_\lambda \frac{\left|\sum_{vc\mathbf{k}} A_\lambda^{vc\mathbf{k}} \tilde{\rho}_{vc\mathbf{k}}(\mathbf{q})\right|^2}{\omega - E_\lambda + i\eta}, \quad (9)$$

where $\Omega$ is the crystal volume, and the oscillator strengths are $\tilde{\rho}_{vc\mathbf{k}}(\mathbf{q}) = \int \varphi^*_{v\mathbf{k}-\mathbf{q}}(\mathbf{r}) e^{-i\mathbf{q}\cdot\mathbf{r}} \varphi_{c\mathbf{k}}(\mathbf{r}) d\mathbf{r}$, where $\varphi_{v/c\mathbf{k}}(\mathbf{r})$ are KS orbitals. With respect to the independent-particle approximation (IPA) where the electron-hole interactions are neglected, peaks in the BSE absorption spectra are located at the exciton energies $E_\lambda$, instead of $E_{vc\mathbf{k}}$, and have modified intensities resulting from the mixing of the oscillator strengths that are modulated by the excitonic coefficients $A_\lambda^{vc\mathbf{k}}$. In this context, the exciton binding energy $E_b$ is defined as the energy difference between the minimum direct gap energy $E_{vc\mathbf{k}}$ and the exciton energy $E_\lambda$.

The two-particle correlation function between an electron and a hole is

$$\Psi_\lambda(\mathbf{r}_h, \mathbf{r}_e) = \sum_{vc\mathbf{k}} A_\lambda^{vc\mathbf{k}} \varphi^*_{v\mathbf{k}}(\mathbf{r}_h) \varphi_{c\mathbf{k}}(\mathbf{r}_e). \quad (10)$$

*Spectra at finite temperature*

To account for temperature and nuclear quantum effects in the spectra we perform the averaging over independent configurations sampled with NVT-Smart Monte Carlo. Following Ref. [10] we perform the quantum averaging (QA), which considers only direct transitions between pairs of electronic states of quantum or thermally averaged bands taking into account only nuclear zero point motion and thermal renormalizations of the bands, but neglecting phonon-assisted transitions. This procedure differs from the conventional semi-classical averaging introduced by Williams [11] and Lax [12] (WL), which substitutes the spectrum of nuclear excitation with a continuum. However, for light nuclei such as hydrogen, replacing the nuclear spectrum by a classical continuum might not be accurate enough in the temperature regime explored by experiments. In WL the dielectric function is obtained for each nuclear configuration $\mathbf{R}$ and then averaged over independent configurations

$$\epsilon^{WL}(\omega, T) = \langle \epsilon^{\mathbf{R}}(\omega) \rangle. \quad (11)$$

In QA instead we average independently $E_\lambda$ and spectral strength $P_\lambda \equiv \left|\sum_{vc\mathbf{k}} A_\lambda^{vc\mathbf{k}} \tilde{\rho}_{vc\mathbf{k}}(\mathbf{q})\right|^2$ computed for each configuration. Considering that this quantities are computed for different nuclear configurations $\mathbf{R}$ and inserting it into Eq. 9 we get

$$\epsilon^{QA}(\omega, T) = 1 - \lim_{\mathbf{q}\to 0} \frac{8\pi}{\Omega q^2} \sum_\lambda \frac{\langle P_\lambda^{\mathbf{R}} \rangle}{\omega - \langle E_\lambda^{\mathbf{R}} \rangle + i\eta}. \quad (12)$$

Figure 6 shows the comparison between quantum (QA) and quasiclassical (WL) averaging for two compressions and compare with experimental measurements. We observe that the spectra overall are similar, except at the onset, especially at low pressure, where the WL averaging has a shoulder below the optical gap (black vertical line). This low energy shoulder in WL should approximate the phonon-assisted transitions. The onset of QA also agrees better with the experimental onset at low pressure.

Figure 7 shows the BSE and independent particle (IPA) GW absorption spectra at the lowest ($\rho/\rho_0 = 3.15$) and highest ($\rho/\rho_0 = 8.48$) compressions. The spectra are shown in the WL approximation due to technical details of the calculations. Note that the IPA-GW spectra are converged at higher energy (we show only converged

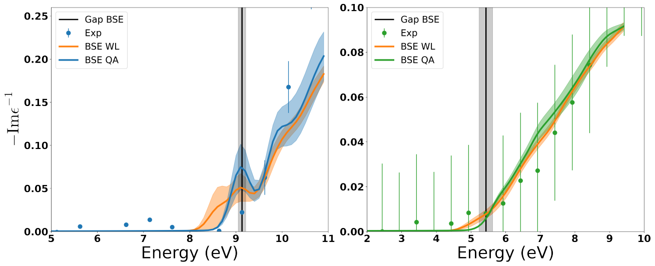


FIG. 6. Electron energy loss spectra. Semiclassical vs quantum averaging predictions at $\rho/\rho_0 = 3.15$ compared to experiments at $\rho/\rho_0 = 3.34$(left) and at $\rho/\rho_0 = 8.48$ compared to experiments at $\rho/\rho_0 = 8.63$ (right).

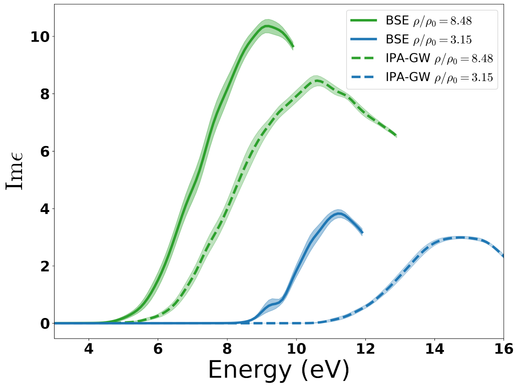


FIG. 7. Absorption spectra at $\rho/\rho_0 = 3.15$ (blue) and $\rho/\rho_0 = 8.48$ (green). The spectra are obtained from the solution of the BSE (solid lines) and from the IPA-GW (dashed lines) with e-h interactions neglected. We observe a sharper excitonic onset at $\rho/\rho_0 = 3.15$ with BSE, not present in the GW spectra without excitonic effects. At $\rho/\rho_0 = 8.48$ the onset (at 5eV) is rather weak.

part). The IPA-GW spectra comprise interband transitions and mark the onset of the continuum. Below the IPA-GW onset, the absorption spectra consist of excitons.

*Computational details*

In this section we report the details of the electron energy loss and absorption spectra calculations. We have performed $G_0W_0$ and BSE calculations on 10 independently sampled configurations to obtain the renormalized spectra due to nuclear temperature and quantum effects. We have calculated the loss spectra for the lowest ($\rho/\rho_0 = 3.15$) and highest ($\rho/\rho_0 = 8.48$) compression.

LDA and GW calculations were carried out with ABINIT [30], while EXC code [31] was used for BSE calculations.

The KS ground-state calculation, in the local density approximation (LDA), converged with an energy cutoff of 130 Hartree and a $4\times4\times4$ **k**-point grid of the supercell.

In the perturbative $G_0W_0$ calculations, the dielectric matrix with a cutoff energy of 7.4 Hartree was computed within the RPA with LDA energies, using a $4 \times 4 \times 4$ **k**-point grid and 500 bands, while the self-energy required 380 bands and 32 Hartree cutoff energy. $G_0W_0$ is a standard method that is shown to be accurate to describe quasiparticle gaps of solids [32].

The BSE hamiltonian, (Eq. (8) of SM), has been built, following the standard approach, using results from the perturbative $G_0W_0$ calculations to scissor-correct the LDA energies (computed individually for each configuration) and a statically screened Coulomb interaction $W$ calculated in RPA.

Convergence with the number of bands of the energy loss spectra for different independent configurations at each compression is illustrated in Fig. 8. The left panels of Fig. 8 show the convergence of two configurations at $\rho/\rho_0 = 3.15$. With 80 bands (48 valence and 32 conduction) the convergence is satisfactory up to $\sim$11 eV. Most important, the energy of the first peak (or of the onset) of the spectra does not change, indicating the convergence of the optical gap. The first peak for both configurations at low pressure convergence slowly and in non-monotonic fashion, which is due to the different convergence of the real $\epsilon_1$ and imaginary $\epsilon_2$ parts of the dielectric function that make the final spectra (see Eq. 6). The first peak in $\epsilon_2$ slowly decreases with the number of bands and $\epsilon_1$ at the same energy is close to zero, this makes the final first peak in the loss spectra to increase. The statistical uncertainty of the first peak is rather large, the underconvergence might add some systematic uncertainty in intensity, but will not change the position of the onset. At higher compression $\rho/\rho_0 = 8.48$ on the right panels of Fig. 8 the convergence is much faster and is reached at $\sim$8 eV with 80 bands (48 valence and 32 conduction). Similar convergence trend is seen in the absorption spectra on figure 9. Here it is important to note that the maximum of the spectrum is at $\sim$11eV independently of the number of bands. We associate this peak to the second excitation of the independent molecule (see Fig. 3 of the main text).

Figure 10 shows the convergence of the loss function with respect to the **k**-points grid at the highest compression. We can see that already for a $4 \times 4 \times 4$ grid the spectrum is converged (note also that the calculations are performed in the supercell). At lower compression, where molecules are more isolated and insulating properties are more pronounced, convergence with respect to **k**-points occurs faster.

The BSE calculations at different pressures and for many configurations are feasible due to the use of the electronic screening $W$ (see Eq. 8) computed for only one configuration at each pressure. This means that the BSE calculations for different configurations are performed using the screening of another configuration at the same

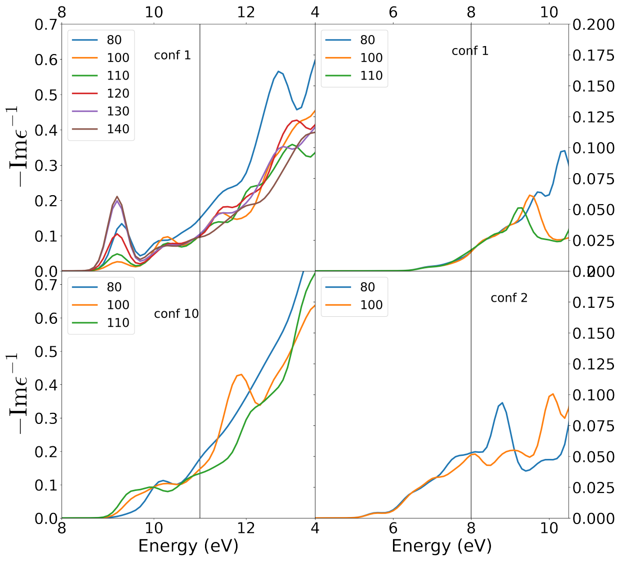


FIG. 8. Electron energy loss spectra dependence on the number of bands for a single configuration at $\rho/\rho_0 = 3.15$ (left, top) and $\rho/\rho_0 = 8.48$ (right, top) and for a second configuration at $\rho/\rho_0 = 3.15$ (left, bottom) and $\rho/\rho_0 = 8.48$ (right, bottom). In this article we use spectra with 80 bands, all valence bands are considered; for energies below the vertical lines the changes in the spectra are in the order of the statistical uncertainty due to the configurational averaging.

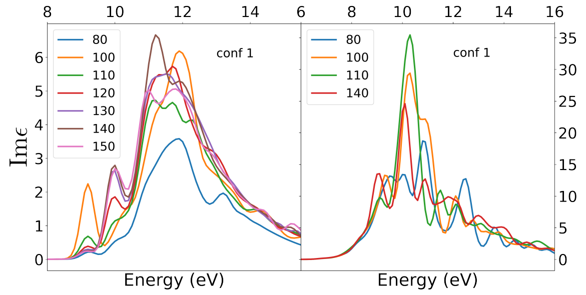


FIG. 9. Convergence of the imaginary part of dielectric function with the number of bands for a single configuration at $\rho/\rho_0 = 3.15$ (left) and $\rho/\rho_0 = 8.48$ (right).

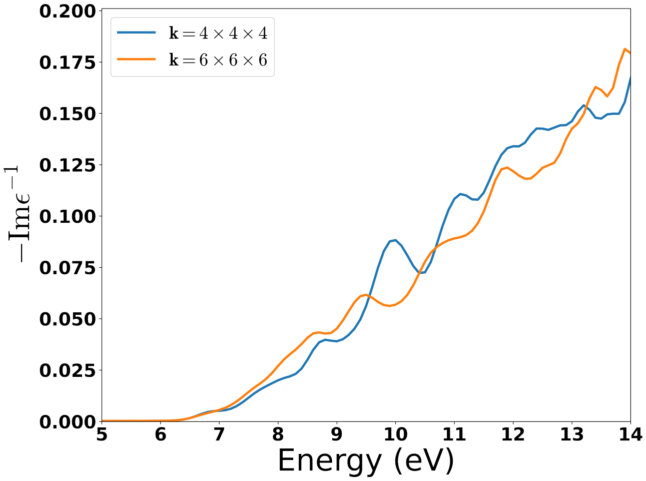


FIG. 10. Electron energy loss spectra for one configuration at $\rho/\rho_0 = 8.48$. Convergence with k-points. We assume that at lower pressure, where the molecules are more isolated, the convergence is faster. Note that the number of bands was reduced to 28 valence and 32 conduction bands to afford the large k calculations.

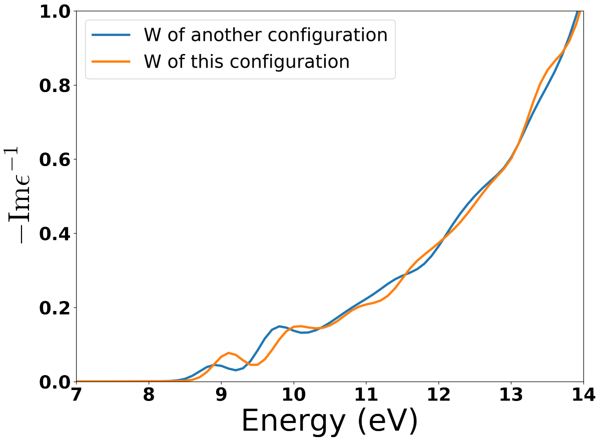


FIG. 11. Electron energy loss spectra for one configuration at $\rho/\rho_0 = 3.15$ obtained with BSE and GW using electron screening $W$ of another configuration at the same density (blue) of the current configuration (orange)

pressure. Figure 11 demonstrates the validity of this approximation for one configuration at 5 GPa. The orange spectra is obtained with $W$ computed for the same configuration, the blue spectra is obtained with $W$ computed for another configuration. The two spectra agree within the uncertainty range of the final spectra on Fig. 2 and 3 of the main text. The reason for the validity of this approximation is that $W$ is long-ranged and depends on the collective behaviour of electrons and is not sensitive to the local changes of the structure [33].

*Electron loss for zero and finite momentum transfer*

The BSE calculations were done at zero momentum transfer to have a direct comparison with QMC results. Experimental measurements [34] are performed at finite momentum transfer at $q = 4\pi \sin(\theta)/\lambda$, where $\theta = 15°$ is the scattering angle and $\lambda = 10^4$ eV $= 1.24$ Å is the incident x-ray wavelength, which makes $q = 2.63$ Å$^{-1}$. We have compared theoretical spectra at zero and at finite $\mathbf{q}$ for a selected configuration at each compression. To account for the random orientation of hydrogen crys-

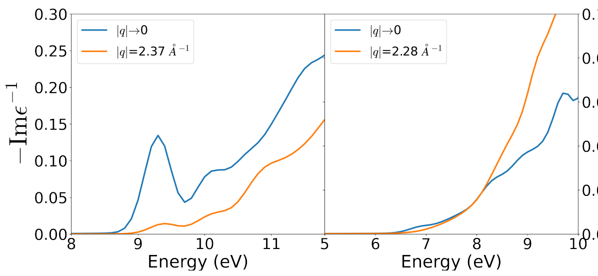


FIG. 12. Electron energy loss spectra for a single configuration at $\rho/\rho_0 = 3.15$ (left) and $\rho/\rho_0 = 8.48$ (right) obtained with BSE at zero momentum transfer (blue) and at finite momentum transfer close to the experimental value (orange).

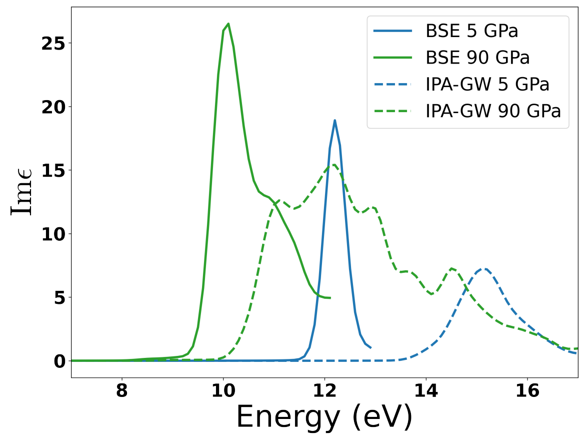


FIG. 13. BSE and IPA-GW absorption spectra for the relaxed (ideal) $P6_3/m$ structure at $P_{wdW-DF1}(T=0) = 5$GPa and 90 GPa. Pressure values obtained with wdW-DF1 DFT functional. The Gaussian broadening is 0.2 eV.

tals in experiment we will average over $\mathbf{q} = (q_x, 0, 0)$, $\mathbf{q} = (0, q_y, 0)$ and $\mathbf{q} = (0, 0, q_z)$. Figure 12 shows the comparison for one configuration at low (left panel) and high (right panel) compression between the loss spectra at vanishing momentum (blue) and at close to experimental momentum (orange). At high compression the difference is small up to 8.5 eV (which is the convergence limit) and the position of the onset is unchanged. At low compression, the difference is more pronounced, however, the position on the onset is changed by only $\sim$0.1 eV. Note that we do not have absolute intensities of the experimental spectra, which makes the slope of the onsets less important for comparison.

### *Absorption spectra for ideal structures*

Figure 13 shows the absorption spectra at highest and lowest compression for the relaxed (ideal) $P6_3/m$ structure using BSE (with excitonic effects) and within the IPA-GW. The structures correspond to the ones used in QMC (see Fig. 4 of the main text). At low pressure single excitonic peak indicates a molecular nature of the excitation. At high pressure, the first excitonic peak with the highest intensity indicates that the molecular nature of the excitation is preserved, contrary to the quantum crystal, where excitonic effects are small and almost indistinguishable from the continuum IPA-GW spectra (see Fig. 7). Interestingly, the binding energies are comparable to the once of quantum crystals, e.g. 1.7 eV at $\sim$ 5 GPa and 0.5 eV at $\sim$ 90 GPa. The nuclear quantum and temperature effects shift the spectrum to lower energies by a constant amount of $\sim$ 3 eV irrespective of compression. Moreover those effect are responsible for a broadening of the main excitonic peak, the amount of which increases with pressure. We can conclude that, even though the neutral and quasiparticle gaps shift rigidly to lower energies due to nuclear effects, the spectral shape is affected differently at different densities.

### *Excitonic wave function*

Figure 14 shows, for fixed nuclear configurations, the nature of the spatial distribution of the lowest energy exciton wave function (Eq. 10). The hole position is integrated over, resulting in electron density $\int d\mathbf{r}_h |\Psi_0(\mathbf{r}_h, \mathbf{r}_e)|^2$. Since the hole position will be mostly located at the molecular centers, we evaluate the integral as a sum of electron densities with the hole position in the center of each molecule (total of 48 points). We can see that whereas the exciton at the lowest compression is entirely localised on the longest molecule, at $\rho/\rho_0 = 4.47$ the exciton reaches to nearby molecules and becomes more delocalized. At the highest compression, the exciton is completely delocalized over the supercell and goes from Frenkel molecular to a Wannier-like exciton.


[1] P. Loubeyre, R. LeToullec, D. Hausermann, M. Hanfland, R. J. Hemley, H. K. Mao, and L. W. Finger, X-ray diffraction and equation of state of hydrogen at megabar pressures, Nature **383**, 702 (1996).

[2] M. Holzmann, D. M. Ceperley, C. Pierleoni, and K. Esler, Backflow correlations for the electron gas and metallic hydrogen, Physical Review E **68**, 046707 (2003), arXiv:0304165 [cond-mat].

[3] C. Pierleoni, K. T. Delaney, M. A. Morales, D. M. Ceperley, and M. Holzmann, Trial wave functions for high-pressure metallic hydrogen, Computer Physics Communications **179**, 89 (2008), arXiv:0712.0161.

[4] P. Giannozzi, S. Baroni, N. Bonini, M. Calandra, R. Car, C. Cavazzoni, D. Ceresoli, G. L. Chiarotti, M. Cococcioni, I. Dabo, A. D. Corso, S. de Gironcoli, S. Fabris,

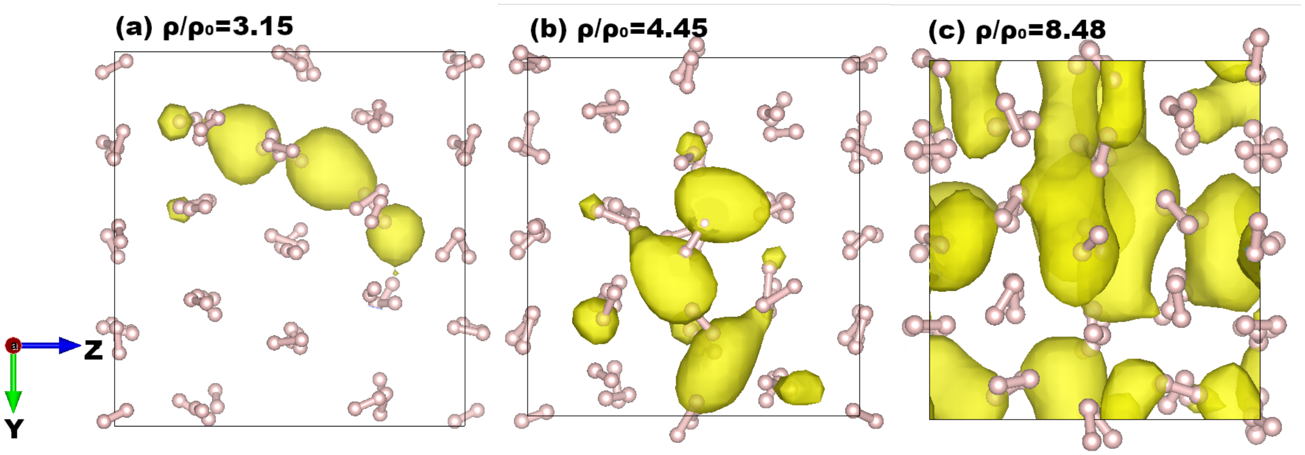


FIG. 14. Spatial distribution of the lowest energy exciton wave function integrated over the hole position $\mathbf{r}_h$: $\int d\mathbf{r}_h|\Psi_0(\mathbf{r}_h,\mathbf{r}_e)|^2$, see Eq. 10, obtained from BSE calculations for one configuration at different compressions: $\rho/\rho_0 = 3.15$ (left), $\rho/\rho_0 = 4.45$ (middle) and $\rho/\rho_0 = 8.48$ (right). The isosurface level is 10%.


G. Fratesi, R. Gebauer, U. Gerstmann, C. Gougoussis, A. Kokalj, M. Lazzeri, L. Martin-Samos, N. Marzari, F. Mauri, R. Mazzarello, S. Paolini, A. Pasquarello, L. Paulatto, C. Sbraccia, S. Scandolo, G. Sclauzero, A. P. Seitsonen, A. Smogunov, P. Umari, and R. M. Wentzcovitch, QUANTUM ESPRESSO: a modular and open-source software project for quantum simulations of materials, Journal of Physics: Condensed Matter **21**, 395502 (2009).

[5] P. Giannozzi, O. Andreussi, T. Brumme, O. Bunau, M. B. Nardelli, M. Calandra, R. Car, C. Cavazzoni, D. Ceresoli, M. Cococcioni, N. Colonna, I. Carnimeo, A. D. Corso, S. de Gironcoli, P. Delugas, R. A. DiStasio, A. Ferretti, A. Floris, G. Fratesi, G. Fugallo, R. Gebauer, U. Gerstmann, F. Giustino, T. Gorni, J. Jia, M. Kawamura, H.-Y. Ko, A. Kokalj, E. KÃŒçÃŒkbenli, M. Lazzeri, M. Marsili, N. Marzari, F. Mauri, N. L. Nguyen, H.-V. Nguyen, A. O. de-la Roza, L. Paulatto, S. Poncé, D. Rocca, R. Sabatini, B. Santra, M. Schlipf, A. P. Seitsonen, A. Smogunov, I. Timrov, T. Thonhauser, P. Umari, N. Vast, X. Wu, and S. Baroni, Advanced capabilities for materials modelling with quantum ESPRESSO, Journal of Physics: Condensed Matter **29**, 465901 (2017).

[6] M. Morales, R. Clay, C. Pierleoni, and D. Ceperley, First Principles Methods: A Perspective from Quantum Monte Carlo, Entropy **16**, 287 (2013).

[7] C. Pierleoni, M. a. Morales, G. Rillo, M. Holzmann, and D. M. Ceperley, Liquid–liquid phase transition in hydrogen by coupled electron–ion Monte Carlo simulations, Proceedings of the National Academy of Sciences **113**, 4954 (2016).

[8] Y. Yang, V. Gorelov, C. Pierleoni, D. M. Ceperley, and M. Holzmann, Electronic band gaps from Quantum Monte Carlo methods, Physical Review B **101**, 85115 (2020), arXiv:1910.07531.

[9] V. Gorelov, M. Holzmann, D. M. Ceperley, and C. Pierleoni, Energy Gap Closure of Crystalline Molecular Hydrogen with Pressure, Physical Review Letters **124**, 116401 (2020), arXiv:1911.06135.

[10] V. Gorelov, D. M. Ceperley, M. Holzmann, and C. Pierleoni, Electronic structure and optical properties of quantum crystals from first principles calculations in the Born-Oppenheimer approximation, J. Chem Phys **153**, 234117 (2020), arXiv:2010.01988.

[11] F. E. Williams, An absolute theory of solid-state luminescence, The Journal of Chemical Physics **19**, 457 (1951).

[12] M. Lax, The franck-condon principle and its application to crystals, The Journal of Chemical Physics **20**, 1752 (1952).

[13] V. Gorelov, Y. Yang, M. Ruggeri, D. M. Ceperley, C. Pierleoni, and M. Holzmann, Neutral band gap of carbon by quantum monte carlo methods, Condensed Matter Physics **26**, 33701 (2023).

[14] J. H. Constable, C. F. Clark, and J. R. Gaines, The dielectric constant of H2, D2, and HD in the condensed phases, Journal of Low Temperature Physics **21**, 599 (1975).

[15] R. J. Hunt, M. Szyniszewski, G. I. Prayogo, R. Maezono, and N. D. Drummond, Quantum Monte Carlo calculations of energy gaps from first principles, Physical Review B **98**, 1 (2018), arXiv:1806.04750.

[16] A. Annaberdiyev, G. Wang, C. A. Melton, M. C. Bennett, and L. Mitas, Phys. Rev. B **103**, 205206 (2021).

[17] R. M. Martin, L. Reining, and D. M. Ceperley, *Interacting Electrons* (Cambridge University Press, Cambridge, 2016).

[18] D. M. Ceperley and B. J. Alder, Ground state of solid hydrogen at high pressures, Physical Review B **36**, 2092 (1987).

[19] G. Onida, L. Reining, and A. Rubio, Electronic excitations: density-functional versus many-body Green's-function approaches, Reviews of Modern Physics **74**, 601 (2002).

[20] G. Strinati, Rivista del Nuovo Cimento **11**, 1 (1988), and references therein.

[21] S. L. Adler, Quantum theory of the dielectric constant in real solids, Phys. Rev. **126**, 413 (1962).

[22] N. Wiser, Dielectric constant with local field effects included, Phys. Rev. **129**, 62 (1963).

[23] L. Hedin, New method for calculating the one-particle green's function with application to the electron-gas problem, Phys. Rev. **139**, A796 (1965).

[24] M. S. Hybertsen and S. G. Louie, Electron correlation in semiconductors and insulators: Band gaps and quasiparticle energies, Phys. Rev. B **34**, 5390 (1986).

[25] R. W. Godby, M. Schlüter, and L. J. Sham, Self-energy operators and exchange-correlation potentials in semiconductors, Phys. Rev. B **37**, 10159 (1988).

[26] S. Albrecht, L. Reining, R. Del Sole, and G. Onida, Ab initio calculation of excitonic effects in the optical spectra of semiconductors, Phys. Rev. Lett. **80**, 4510 (1998).

[27] L. X. Benedict, E. L. Shirley, and R. B. Bohn, Optical absorption of insulators and the electron-hole interaction: An ab initio calculation, Phys. Rev. Lett. **80**, 4514 (1998).

[28] M. Rohlfing and S. G. Louie, Electron-hole excitations and optical spectra from first principles, Phys. Rev. B **62**, 4927 (2000).

[29] V. Gorelov, L. Reining, M. Feneberg, R. Goldhahn, A. Schleife, W. R. L. Lambrecht, and M. Gatti, Delocalization of dark and bright excitons in flat-band materials and the optical properties of V2O5, npj Computational Materials **8**, 94 (2022).

[30] X. Gonze, G.-M. Rignanese, M. Verstraete, J.-M. Beuken, Y. Pouillon, R. Caracas, F. Jollet, M. Torrent, G. Zerah, M. Mikami, *et al.*, A brief introduction to the abinit software package, Z. Kristallogr **220**, 558 (2005).

[31] `http://www.bethe-salpeter.org/`.

[32] F. Hüser, T. Olsen, and K. S. Thygesen, Quasiparticle gw calculations for solids, molecules, and two-dimensional materials, Phys. Rev. B **87**, 235132 (2013).

[33] V. Gorelov, L. Reining, W. R. L. Lambrecht, and M. Gatti, Robustness of electronic screening effects in electron spectroscopies: Example of $V_2O_5$, Physical Review B **107**, 075101 (2023).

[34] B. Li, Y. Ding, D. Y. Kim, L. Wang, T.-C. Weng, W. Yang, Z. Yu, C. Ji, J. Wang, J. Shu, J. Chen, K. Yang, Y. Xiao, P. Chow, G. Shen, W. L. Mao, and H.-K. Mao, Probing the Electronic Band Gap of Solid Hydrogen by Inelastic X-Ray Scattering up to 90 GPa, Physical Review Letters **126**, 36402 (2021).
